# Supplementary material for: Theoretical bounds on estimation error for meta-learning
Source: arXiv:2010.07140 source file (2020-10-14)
Supplement: Supplementary file 6 [file notation.tex]

\section{Notation}
\label{app:notation}

\begin{table}[h]
    \centering
    \noindent\setlength\tabcolsep{4pt}%\setlength{\extrarowheight}{5pt}%
    \begin{tabular}{c|l}
         &  \textbf{Description} \\\hline
        $\spaceX$ & The domain of the data, e.g. $\bbR^d$ \\
        $\spaceY$ & The range of the data, e.g. $\bbR$ \\
        $\spaceZ$ & The product space $\spaceX \times \spaceY$ \\
        $\calP$ & A collection of distributions over $\spaceZ$ \\
        $\calJ$ & A (finite) subset of distributions in $\calP$ \\
        $P$ & An element of $\calP$\\
        $P^k$ & The product distribution, whose samples correspond to $k$ independent draws from $P$\\
        $P_{1:M}$ & The product distribution, $\Pi_{i=1}^{M} P_i$, for $P_i \in \calP$\\
        $\bar{P}_{1:M}$ & The mixture distribution, $\frac{1}{M}\sum_{i=1}^M P_i$, for $P_i \in \calP$\\
        $\Omega$ & A metric space, containing parameters for each distribution\\
        $\theta$ & A functional, mapping distributions in $\calP$ to parameters in $\Omega$ \\
        $\estimator$ & An estimator $\estimator: \spaceZ^n \rightarrow \calF$\\ 
        $S, \testS$ & Denotes training datasets drawn \iid from some $P \in \calP$.\\&Typically $S = \{z_1,\ldots,z_n\}$,$\testS = \{z'_1,\ldots,z'_k\}$\\
        $S_\calP$ & Denotes a meta-training set drawn \iid from $P_{1:M}$\\
        $[N]$, for $N \in \bbN$ & Indicates the set $\{1,\ldots,N\}$\\
        $\bball_p(r)$ & The $p$-norm ball of radius $r$, centered at $0$.
    \end{tabular}
    \caption{Summary of notation used in this manuscript}
    \label{tab:notation}
\end{table}
